# Supplementary material for: Feature Descriptors for Tracking by Detection: a Benchmark
Source: arXiv:1607.06178 source file (2016-07-21)
Supplement: Supplementary file 1 [file additional.tex]

\section{Additional}

\todo[inline]{Please note this is a collection of tables and images that will not end in the paper. They are good anyway to have a picture of the results}

\begin{figure*}
\centerline{%
	\subfigure{
		\includegraphics[width=0.5\linewidth]{imgs/brisk_correlation.pdf}~
		\includegraphics[width=0.5\linewidth]{imgs/orb_correlation.pdf}~
		}}
\vspace{-2.0mm}
\centerline{%
\subfigure{
		\includegraphics[width=0.5\linewidth]{imgs/akazec_correlation.pdf}~
		\includegraphics[width=0.5\linewidth]{imgs/sift_correlation.pdf}~
		}}
\vspace{-2.0mm}
\addtocounter{subfigure}{-1}
\centerline{%
	\subfigure{	
		\includegraphics[width=0.5\linewidth]{imgs/surf_correlation.pdf}~
		\includegraphics[width=0.5\linewidth]{imgs/cuda_sift_correlation.pdf}~
\label{fig:exp_d}		
}}
\vspace{-2.0mm}
\caption{Correlations matrices between the different evaluated measures of the feature descriptors.}
\vspace{-2mm}
\label{fig:depth_comparison_second}
\end{figure*}

\begin{figure*}[t]
\centerline{% 
		\includegraphics[width=0.98\linewidth]{tables/test.pdf}}
    \vspace{-2mm} 
	\caption{Overall results of the dataset for true positive matching. This is just a preview it won't be in he paper.}
	\label{fig:learnvsno}
\end{figure*}
